# Supplementary material for: Estimating Buildings' Parameters over Time Including Prior Knowledge
Source: arXiv:1901.07469 source file (2019-02-18)
Supplement: Supplementary file 1 [file Appendix.tex]

\section*{Appendix}
\appendix
 
 \section{Challenges to incorporate the Air-Infiltration and Ventilation}
 
  Our objectives are to map the model parameters with interpretable standardized measures.
